# Supplementary material for: SPOT: SE(3) Pose Trajectory Diffusion for Object-Centric Manipulation
Source: arXiv:2411.00965 source file (2025-05-13)
Supplement: Supplementary file 1 [file supp.tex]

\section{Further Details on Object Pose Tracking}
Our approach relies on object pose from the tracker to generate action plans. Besides RGBD observations, the tracker requires a 3D object model and a 2D detection for the first frame. Here, we describe how to obtain this information during both the training and deployment stages.

\noindent  \textbf{Simulation setup.}
We reconstruct the object mesh from the training demonstration sequence using BundleSDF~\cite{wen2023bundlesdf} and obtain the first frame object mask with SAM6D~\cite{lin2024sam} through RGBD observations and the object mesh.

\noindent  \textbf{Real-world setup.}
We obtain real-world object scans using a consumer-grade device, an iPhone equipped with a camera and LiDAR. For 2D object detection, we employ YOLO-World~\cite{cheng2024yolo}, an open-vocabulary object detection model. It takes as input the RGB image of the scene and task-relevant object names as text prompts and outputs their 2D detections. We leverage ChatGPT to extract task-relevant object names from the task description automatically.
